# Supplementary material for: TLXML: Task-Level Explanation of Meta-Learning via Influence Functions
Source: arXiv:2501.14271 source file (2026-08-25)
Supplement: Supplementary file 1 [file references.tex]

\bibliographystyle{splncs04}
\bibliography{../bib/all,../bib/task_relatedness.bib,../bib/meta_learning.bib,../bib/ecmlpkdd.bib}
